# Supplementary material for: IRIS: Wireless Ring for Vision-based Smart Home Interaction
Source: arXiv:2407.18141 source file (2024-07-25)
Supplement: Supplementary file 1 [file 10-appendix.tex]

\appendix

\section{Appendix}

\subsection{Demos}
We have attached a video demo, as well as more extensive audio demos of the various experimental settings. For the comparisons in table \ref{table:results}, we have included results with different combinations of the target voice, background (BG), and a background voice (BGVoice). We have also included qualitative comparisons against the commercially available solution Krisp\footnote{\url{krisp.ai}} in the folder krisp\_comparisons. The audio was piped directly into Krisp via the BlackHole plugin\footnote{\url{https://github.com/ExistentialAudio/BlackHole}}, and recorded directly from the system output of Krisp.
We have also attached the samples used in the listening study that contains samples processed by CB-UNet, CB-Conv-TasNet, and CB-Net.

\subsection{Hyperparameters and Training Details}

\textbf{Training Parameters} We use a learning rate of $\SI{3e-4}{}$ along with the ADAM optimizer  \cite{kingma2014adam} for training the network. The network was trained on a single Nvidia TITAN Xp GPU. Because of the small size of the network, training could be completed within a single day and generally required ~50 epochs to reach convergence.

\textbf{Data Augmentation} As an additional data augmentation step we make the following perturbations to the data: High-shelf and low-shelf gain of up to $\SI{2}{dB}$ are randomly added using the \texttt{sox} library\footnote{\url{http://sox.sourceforge.net/}}.

\subsection{Additional Figures}

\begin{figure}[h]
\vskip -0.1in
\centering
\includegraphics[width=1\linewidth]{figures/side_voice_figure.png}
\vskip -0.05in
\caption{\small{Background Voice Performance. ClearBuds network uses spatial cues to allow it to separate background voices from the target speaker, even when the background voice is much louder than the target voice. In this time domain view, this is evident in the time window where the target speaker is silent (highlighted). In the mixture (first) the background voice continues to talk. The mono-channel Facebook Denoiser is unable to suppress this background voice without spatial information (second). Our multi-channel network (third) removes the background voice even in this region approaching the ground truth (fourth). From a user experience perspective, this would allow a user to not toggle the mute button on call, even when they are not speaking.}}
\label{fig:network}
\vskip -0.25in
\end{figure}

\begin{figure}[h]
\vskip -0.1in
\centering
\includegraphics[width=0.7\linewidth]{figures/experimental_setup_figure.png}
\vskip -0.05in
\caption{\small{End-to-end system experiment physical set up. A foam mannequin head with a speaker (Sony SBS-XB12) inserted into its artificial mouth uttered one hundred VCTK samples from the test partition.
Ambient environmental sound (from WHAM! dataset) was played via four monitors (PreSonus Eris E3.5) positioned to fill 3 meter by 4 meter room on a 0.75 meter radius circle, and background voice (also VCTK) was played from a monitor positioned 0.4 meters from head on the right.}}
\label{fig:network}
\vskip -0.25in
\end{figure}
